# Supplementary material for: Visualising Deep Network's Time-Series Representations
Source: arXiv:2103.07176 source file (2021-06-17)
Supplement: Supplementary file 1 [file Appendix.tex]

Appendixes should appear before the acknowledgment.
